# Supplementary material for: Modeling the impact of temperature and bird migration on the spread of West Nile virus
Source: arXiv:2508.14740 ancillary file (2025-11-30)
Supplement: Supplementary file 1 [file Supplementary_Material.pdf]

# **Supplementary file:** Modeling the spread of West Nile virus under the influence of temperature and bird migration

Pride Duve, Felix Sauer, and Renke Lühken

Bernhard-Nocht Institute for Tropical Medicine, Hamburg, Germany

## S1: Temperature-space dependent mosquito parameters

Figures (1), (2) and (3) show the temperature-dependent mosquito biting rate $\beta(T, \boldsymbol{x})$, extrinsic incubation period $\gamma_V(T, \boldsymbol{x})$, and the natural mortality rate $\mu_V(T, \boldsymbol{x})$ for each year, whose functions are obtained from [3], [1], and [2] respectively. We observe the differences in the spatial distribution of the values for each year. For example, it can be observed that $\beta(T, \boldsymbol{x})$ is high in the years 2019, 2021, and 2024, as compared to the other years, highlighting the differences in yearly temperatures and their impact on the WNV spreading pattern in Germany. The year 2021 had, on average, a lower mortality, indicating high mosquito activity in most parts of Germany. The extrinsic incubation period is shorter in regions classified by the model as WNV hotspots in 2019, 2021 and 2024.

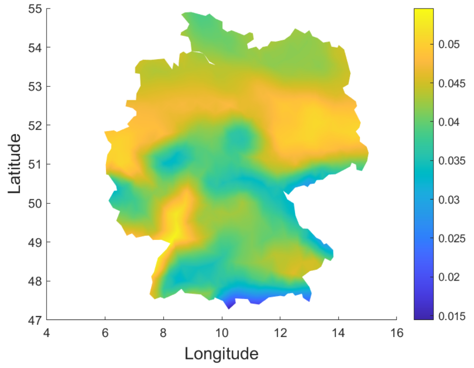


(a) $\beta(T, \boldsymbol{x})$ in 2019.

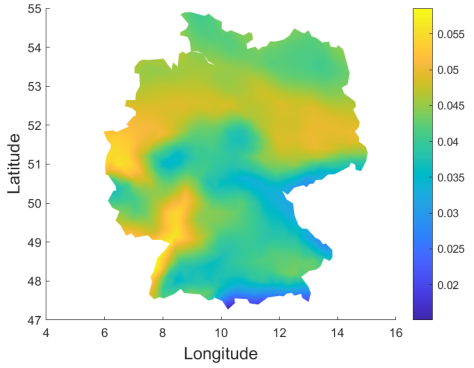


(b) $\beta(T, \boldsymbol{x})$ in 2020.

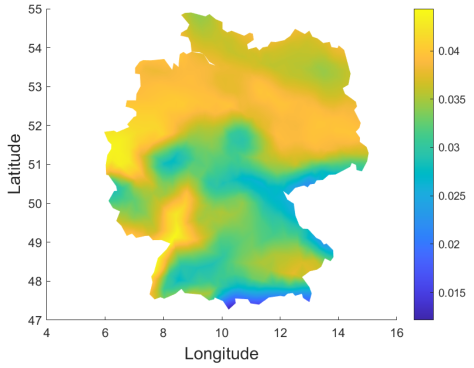


(c) $\beta(T, \boldsymbol{x})$ in 2021.

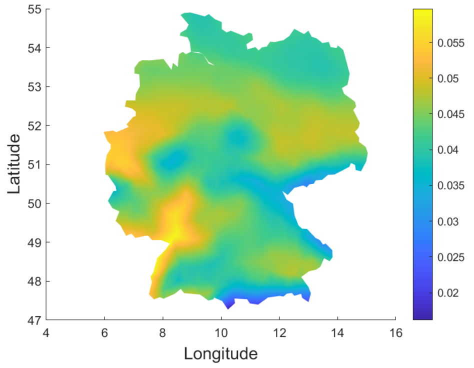


(d) $\beta(T, \boldsymbol{x})$ in 2022.

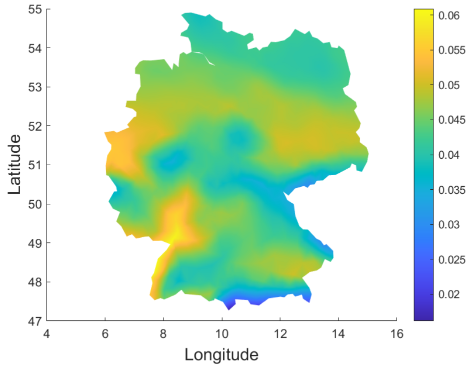


(e) $\beta(T, \boldsymbol{x})$ in 2023.

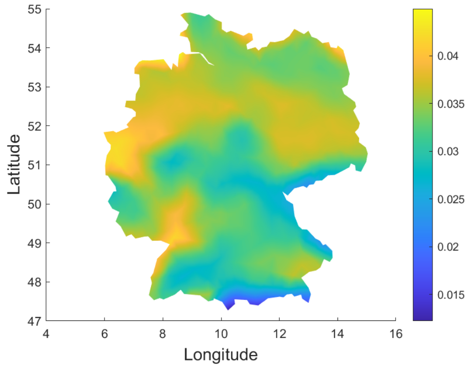


(f) $\beta(T, \boldsymbol{x})$ in 2024.

Figure 1: Temperature and space dependent mosquito biting rate ($\beta(T, \boldsymbol{x})$).

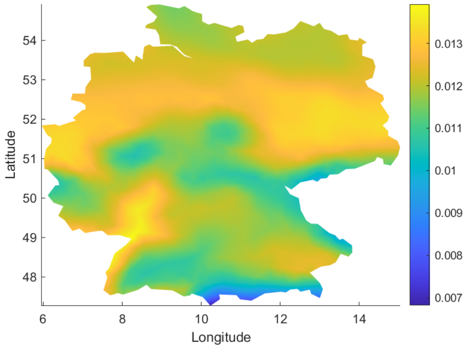


(a) $\gamma_V(T, \boldsymbol{x})$ in 2019.

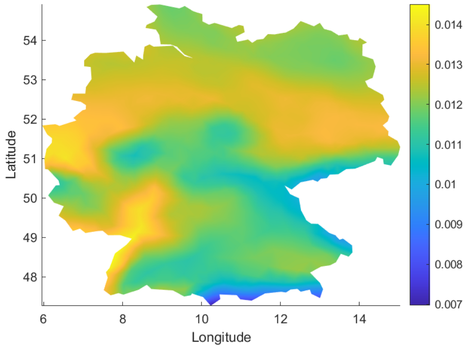


(b) $\gamma_V(T, \boldsymbol{x})$ in 2020.

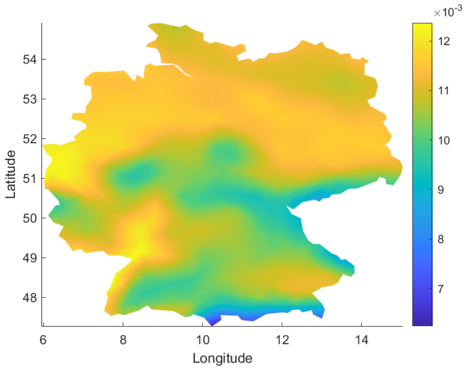


(c) $\gamma_V(T, \boldsymbol{x})$ in 2021.

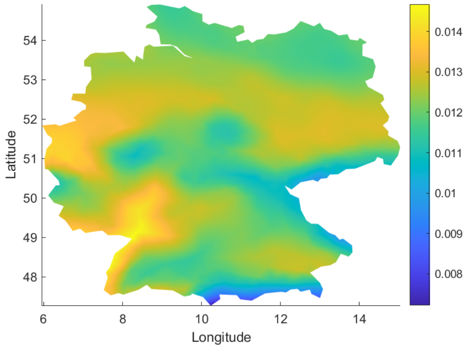


(d) $\gamma_V(T, \boldsymbol{x})$ in 2022.

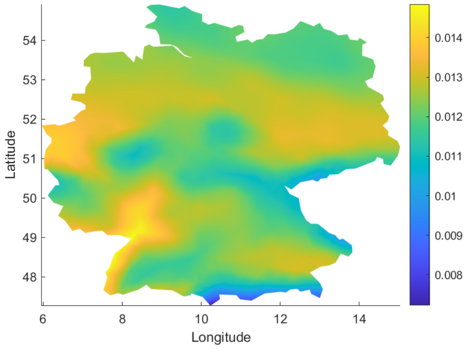


(e) $\gamma_V(T, \boldsymbol{x})$ in 2023.

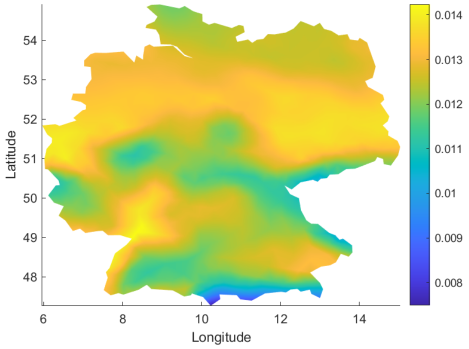


(f) $\gamma_V(T, \boldsymbol{x})$ in 2024.

Figure 2: Temperature and space dependent extrinsic incubation rate $(\gamma_V(T, \boldsymbol{x}))$.

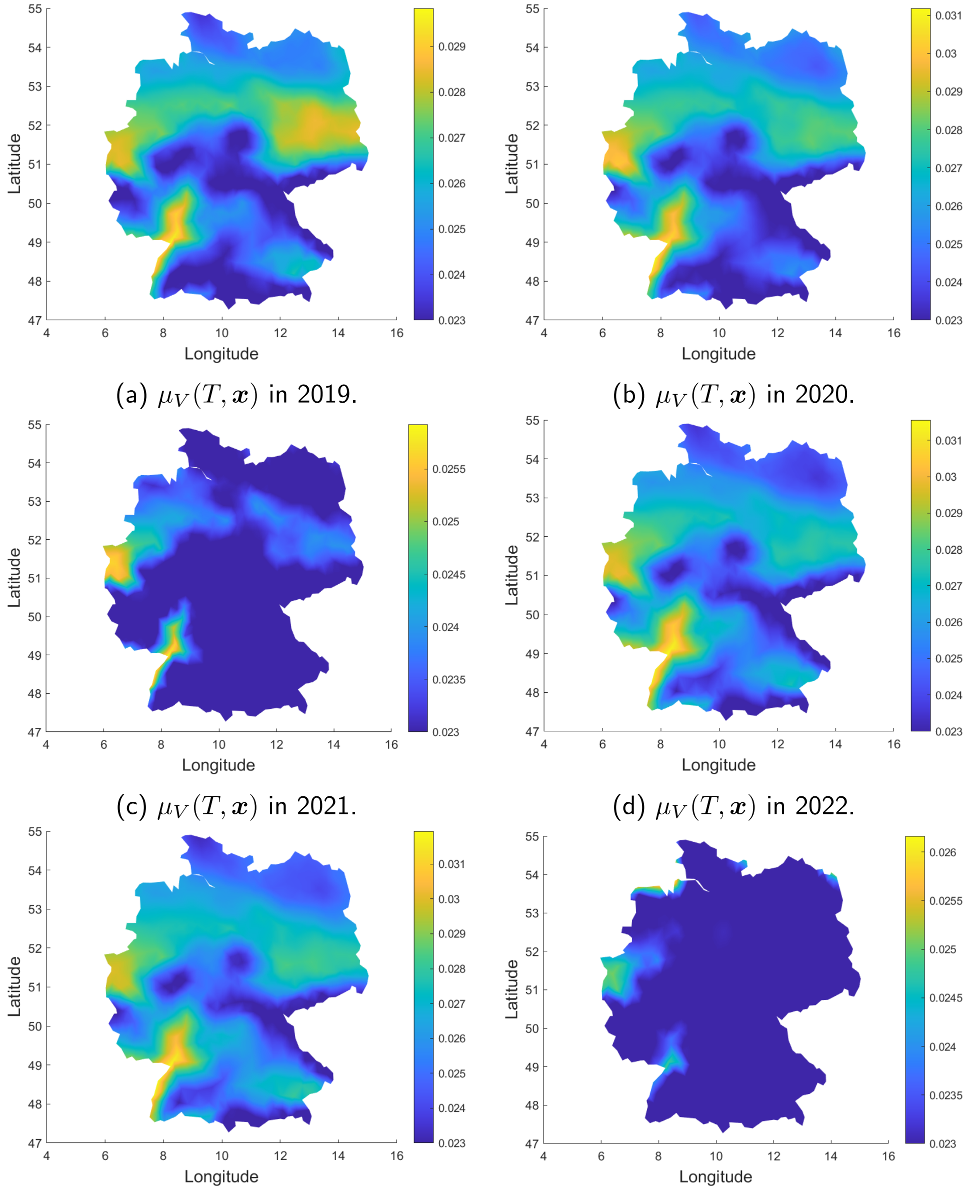


(a) $\mu_V(T, \boldsymbol{x})$ in 2019.

(b) $\mu_V(T, \boldsymbol{x})$ in 2020.

(c) $\mu_V(T, \boldsymbol{x})$ in 2021.

(d) $\mu_V(T, \boldsymbol{x})$ in 2022.

(e) $\mu_V(T, \boldsymbol{x})$ in 2023.

(f) $\mu_V(T, \boldsymbol{x})$ in 2024.

Figure 3: Temperature and space dependent mortality rate ($\mu_V(T, \boldsymbol{x})$).

## S2: Model simulation for the years 2019, 2020 and 2022

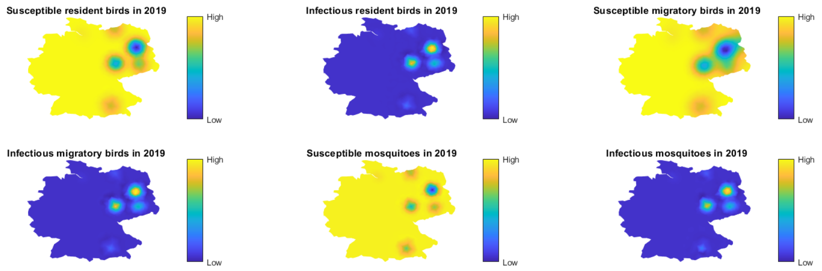


(a) Model simulation for the year 2019.

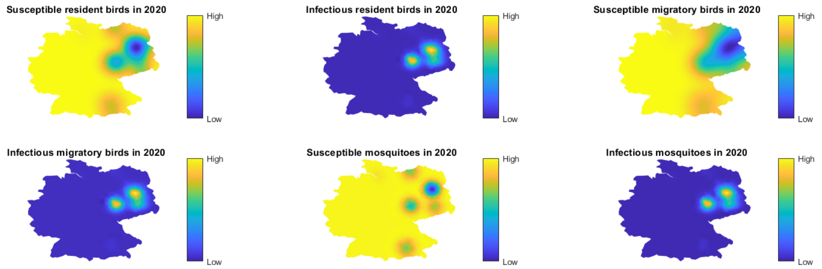


(b) Model simulation for the year 2020.

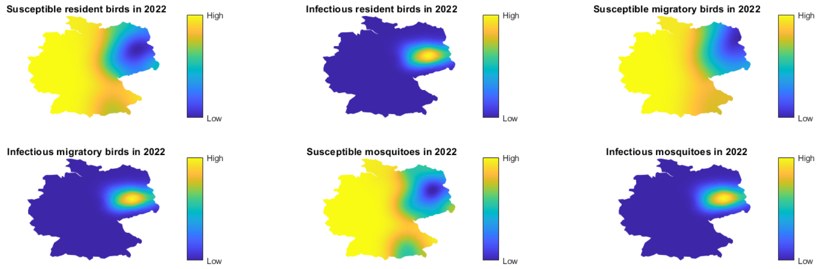


(c) Model simulation for the year 2022.

Figure 4: Model simulation for the years 2019, 2020, and 2022.

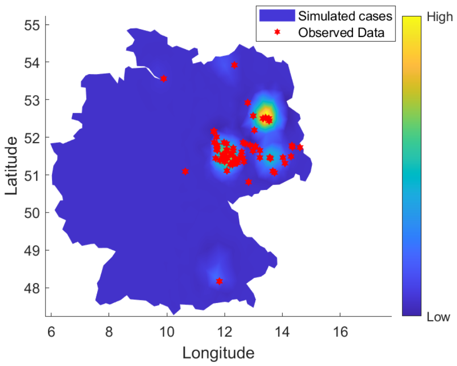


(a) Model simulation for the year 2022.

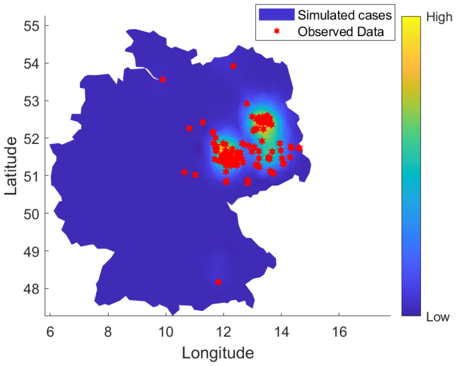


(b) Model simulation for the year 2020.

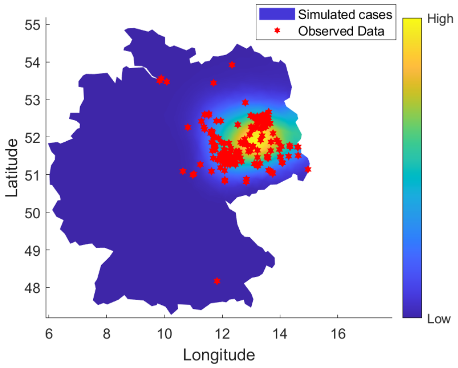


(c) Model simulation for the year 2022.

Figure 5: Model simulation for the years 2019, 2020, and 2022.

Figure (4) shows the model simulation for the years 2019 and 2020, together with observed data.

# S3: 3D hill plots of model simulation

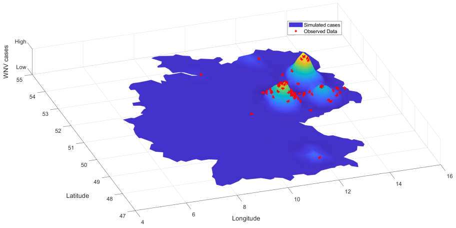


(a) Year 2019.

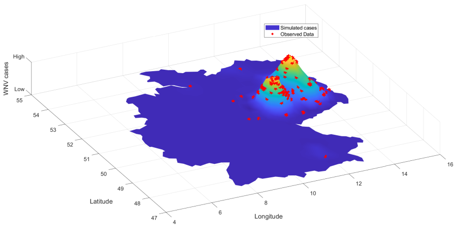


(b) Year 2020.

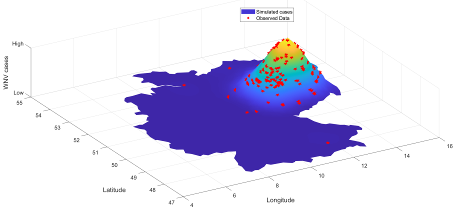


(c) Year 2021.

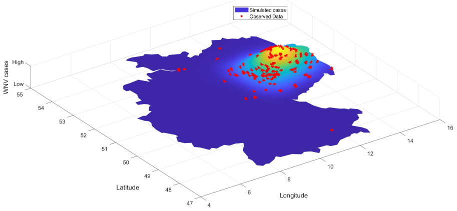


(d) Year 2022.

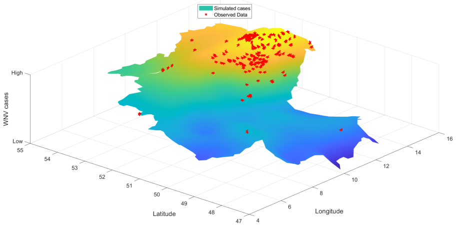


(e) Year 2023.

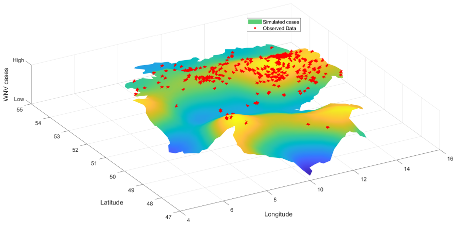


(f) Year 2024.

Figure 6: 3D hill plots of model simulation compared to observed data for the years 2019-2024.

## References

[1] J. Heidecke, J. Wallin, P. Fransson, P. Singh, H. Sjödin, P. C. Stiles, M. Treskova, and J. Rocklöv. Uncovering temperature sensitivity of west nile virus transmission: Novel computational approaches to mosquito-pathogen trait responses. *PLOS Computational Biology*, 21(3):e1012866, Mar. 2025.

[2] V. Laperriere, K. Brugger, and F. Rubel. Simulation of the seasonal cycles of bird, equine and human west nile virus cases. *Preventive Veterinary*

*Medicine*, 98(2–3):99–110, Feb. 2011. https://dx.doi.org/10.1016/j.prevetmed.2010.10.013.

[3] F. Rubel, K. Brugger, M. Hantel, S. Chvala-Mannsberger, T. Bakonyi, H. Weissenböck, and N. Nowotny. Explaining usutu virus dynamics in austria: Model development and calibration. *Preventive Veterinary Medicine*, 85(3–4):166–186, July 2008. https://dx.doi.org/10.1016/j.prevetmed.2008.01.006.
